# Supplementary material for: Provenance in Temporal Interaction Networks
Source: arXiv:2110.05041 source file (2021-10-11)
Supplement: Supplementary file 1 [file Appendix.tex]

\section{Appendix}\label{sec:appendix}
